# Supplementary material for: Stepwise Bose-Einstein condensation in a spinor gas
Source: arXiv:1702.08265 ancillary file (2017-05-26)
Supplement: Supplementary file 1 [file Tc_spinor_resub_SupMat.pdf]

# Supplementary Material for: Stepwise Bose-Einstein Condensation in a Spinor Gas

C. Frapolli,<sup>1</sup> T. Zibold,<sup>1</sup> A. Invernizzi,<sup>1</sup> K. Jimenez-Garcia,<sup>1</sup> J. Dalibard,<sup>1</sup> and F. Gerbier<sup>1</sup>

<sup>1</sup>*Laboratoire Kastler Brossel, Collège de France, CNRS, ENS-PSL Research University, UPMC-Sorbonne Universités, 11 place Marcelin Berthelot, 75005 Paris*

(Dated: May 26, 2017)

## I. EXPERIMENTAL SEQUENCE

### A. Trap geometry

Our experiments start with a thermal gas of  $\sim 10^5$   $^{23}\text{Na}$  atoms in a crossed dipole trap, at a temperature around  $T \approx 4\mu\text{K}$ . We set the normalized magnetization of the cloud  $m_z$  between 0 and 1 using the same procedure as in [1], and perform evaporative cooling by decreasing the power of the optical dipole trap. We found that the magnetization varies during the evaporation ramp, typically by 10–15% (see Section II B below). Once the desired final trap depth is reached, we hold the atoms in the trap for 4 seconds to ensure thermalization. We apply a constant bias magnetic field  $B$  during the evaporation. For the data sets with  $B = 0.1\text{ G}$  and  $B = 0.5\text{ G}$  (resp.  $B = 5.6\text{ G}$ ), the bias field is along the  $\mathbf{x}$  (resp.  $\mathbf{x} + \mathbf{y} + \mathbf{z}$ ) direction (see Fig. 1).

### B. Stern-Gerlach Imaging

We detect the atoms using absorption imaging after a period of expansion in a magnetic field gradient to spatially separate the Zeeman components (Stern-Gerlach – SG – imaging). We use in this work a slightly different SG sequence than in [1, 2]. A quadrupole magnetic field (created by the pair of coils used to operate the magneto-optical trap) together with a strong bias magnetic field parallel to the  $y$  axis produces a magnetic force along  $y$ . We pulse this magnetic force after the trap has been switched off. We trigger a  $\sim 1\text{ ms}$ -long pulse by discharging a large capacitor into the coils. A power diode and a semiconductor switch limit the current pulse to one half

period of the resulting L-C oscillation. After a time of flight of 3 ms, we repump the atoms to the  $F = 2$  hyperfine manifold and take an absorption image using light resonant on the  $F = 2 \rightarrow F' = 3$  transition.

The magnification of the imaging system is calibrated directly by imaging the Kapitza-Dirac diffraction pattern from a pulsed optical lattice with known wavelength, and indirectly by comparison to an orthogonal imaging system calibrated against gravity. Both methods agree within their uncertainty, on the order of 1%.

### C. Trap Calibrations

Evaporative cooling in optical traps is performed by lowering the optical power of the trap laser, which reduces the trap depth but also the trap frequencies [3]. In our experiments, they change from around 2 kHz for the highest power to a few hundred Hz for the lowest. We calibrate the trap frequencies using two methods, (i) center-of-mass oscillations, and (ii) parametric excitation (see Fig. 2). For method (i), we use a gas of atoms polarized in the  $m_F = +1$  Zeeman sublevel ( $m_z \approx 1$ ). We slowly ramp up a magnetic field gradient that displaces the cloud center to a new equilibrium position, and then switch off the gradient to induce oscillations at the trap frequencies. For method (ii), we modulate the dipole trap optical power to induce parametric heating. When interactions can be neglected, resonant excitation is obtained when the modulation frequency coincides with the

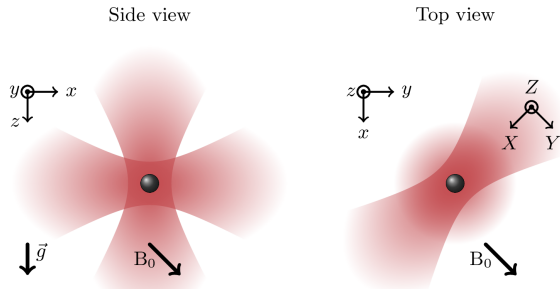

FIG. 1. Crossed dipole trap geometry.

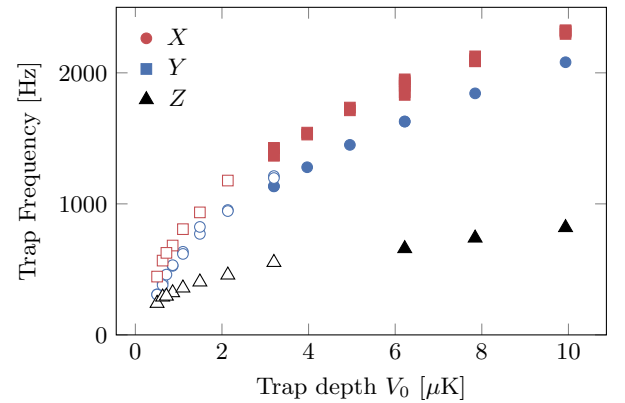

FIG. 2. Evolution of trap frequencies in an evaporation trajectory. Filled symbols indicate frequencies measured with parametric heating, open symbols indicate frequencies measured with dipole oscillations.

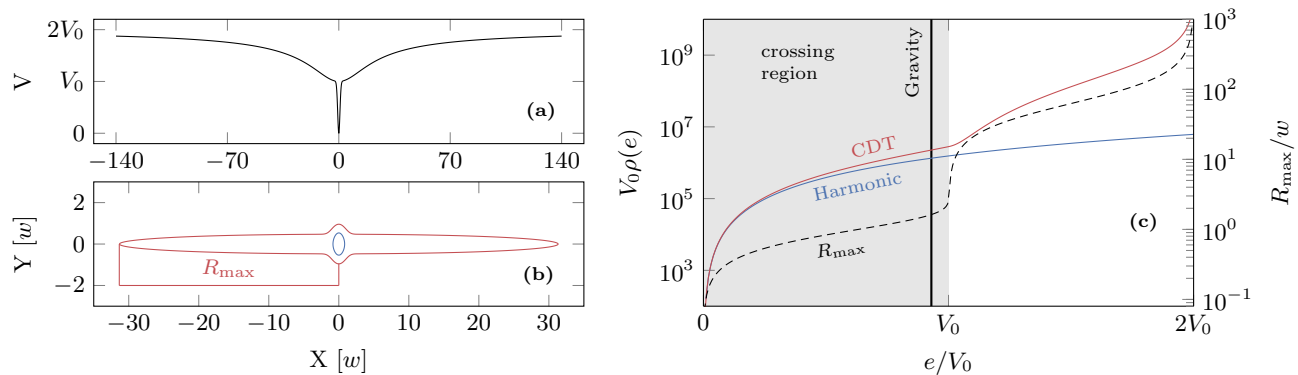

FIG. 3. **a**: Potential  $V$  of a crossed optical dipole trap (CDT) formed by two Gaussian traps of waist  $w$  and trap depth  $V_0$ . **b**: Classical isopotential contours  $V(\mathbf{r}) = E$  for energies  $E < V_0$  (blue solid line) and  $V_0 < E < 2V_0$  (red solid line). **c**: Density of state  $\rho(e)$  (red solid line) and maximum radius of classical trajectory (dashed line). The blue solid line shows the density of states of the harmonic potential closest to the CDT potential  $V(\mathbf{r})$ . The grayed area correspond to classical trajectories bounded within the crossing region. The vertical solid line shows the energy cutoff due gravity for vertical trajectories, slightly lower than the energy  $V_0$  where the atoms escape from the crossing region.

second harmonic of one of the trap frequencies.

Method (i) is best suited for trap frequencies below approximately 1 kHz, and method (ii) above. In our experiment, we cannot switch off the magnetic field gradient faster than approximately a millisecond, which is long compared to the typical oscillation period for the highest trap depths. Consequently, the switch-off becomes almost adiabatic, and the induced oscillations of the center-of-mass are hardly detectable. While the parametric heating method (ii) should in principle work at all temperatures, once a condensate is formed the relation between the measured resonant frequencies and the bare trap frequencies is no longer straightforward. To avoid complicated modelling involving finite temperature theories of Bose-Einstein condensed gases [4], we restrict method (ii) to normal gases above the critical temperature, which corresponds typically to trap frequencies  $\gtrsim 1$  kHz.

## II. EVAPORATION DYNAMICS

### A. Trap Depth

In this Section, we discuss how we extract a trap depth for a crossed dipole trap geometry involving two Gaussian beams, as sketched in Fig. 1. For simplicity we consider here two identical, mutually incoherent beams. The dipole potential for a single beam is [5]  $V(\mathbf{x}) \approx -V_0 e^{-2(x_1^2 + x_2^2)/w^2} / [1 + (x_3/z_R)^2]$ , with  $V_0$  the single-beam trap depth, proportional to laser power, with  $w$  the beam waist and with  $z_R = \pi w^2/\lambda_L$  the Rayleigh length. For the geometry we consider, we have  $x_1 = X, x_2 = Y$  and  $x_3 = Z$  for the vertical beam 1 and  $x_1 = Y, x_2 = Z$  and  $x_3 = X$  for the horizontal beam 2 (see Fig. 3a). For atoms with energies much lower than  $V_0$ , this leads to an approximately harmonic

trap with frequencies  $\omega_{\{X,Y,Z\}} = \{1, \sqrt{2}, 1\} \sqrt{4V_0/mw^2}$ . In general, we distinguish two different energetic regimes based on the shape of the isopotential curves  $V(\mathbf{r}) = E$  (Fig. 3b). For atoms with low energies  $E < V_0$ , the classical trajectories are bounded within the crossing region of size  $\sim w \times w$ . Atoms with energies  $V_0 < E < 2V_0$ , on the other hand, experience classical trajectories extending far in the arms of the CDT, over distances  $\sim R_{\max}$  many times greater than the size of the trapped gas in the crossing region (typically  $\ll w$  for cold clouds with  $k_B T \ll V_0$ ). The high-energy atoms populating the arms of the CDT thus form a very dilute cloud, not necessarily in equilibrium with the majority of atoms in the crossing regions. From this simple picture, the trap depth relevant for evaporative cooling is on the order of  $V_0$ , the energy where the isopotential maximum radius and the density of states  $\rho(E)$  (calculated semiclassically) both increase dramatically (see Fig. 3c). Including gravity, classical trajectories with energies  $\sim V_0 - mgw$  can escape along  $Z$ , as indicated by the vertical line in Fig. 3c.

It is difficult to make more precise statements about the value of  $V_0$ , since it depends on evaporation dynamics, and on the ergodicity of classical trajectories. We did not carry a detailed kinetic calculation of evaporative cooling in the CDT potential  $V(\mathbf{r})$  (as done in [6] for a truncated harmonic trap), a task that goes well beyond the scope of this work. We assume here that we can take  $V_0$  as the relevant trap depth determining the evaporative cooling dynamics. This has no impact on our experimental results, as  $V_0$  is merely used as a label for each point on a given evaporation trajectory.

### B. Discussion on the conservation of magnetization

A typical evaporation trajectory is shown in Fig. 4. The behavior of the total atom number and tempera-

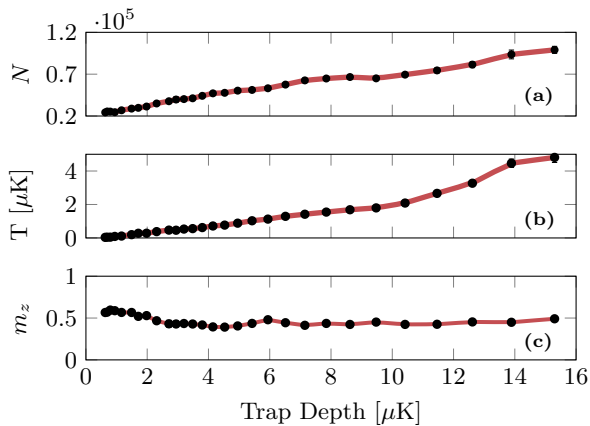

FIG. 4. Evaporation trajectory showing atom number, magnetization and temperature versus trap depth. The solid line shows a numerical interpolation which we use to extract the critical values for each quantity from the critical trap depth (see Section IV).

ture are expected, but one can also notice a variation of the magnetization  $m_z$  with trap depth. This behavior seems at first glance incompatible with the announced conservation law of  $m_z$ . However, the argument that microscopic binary collisions driving the system to thermal equilibrium conserve  $m_z$  disregards the dynamics of evaporative cooling. Once a condensate forms in one of the Zeeman components, evaporation tends to eliminate preferentially atoms in the other Zeeman states.

In spite of this variation, the conservation of magnetization is still relevant to determine the state of kinetic equilibrium reached by the system. The evaporative cooling dynamics is very slow compared to the microscopic thermalization time on which the gas returns to thermal equilibrium. The thermalization time can be estimated from the classical collision time  $1/(n\sigma v_{\text{th}})$  (here,  $n$  is the spatial density of the thermal component,  $\sigma$  the  $s$ -wave scattering cross section,  $v_{\text{th}} = \sqrt{k_B T/\pi m}$  the thermal velocity and  $m$  the mass of a sodium atom). For typical parameters in our experiment, one finds a thermalization time on the order of a ms while typical evaporation times range are around 1 s. As a result, the quantum gases studied in this work can be considered to follow the slowly changing magnetization, with the relevant kinetic equilibrium state at each time determined by a magnetization-conserving Hamiltonian. We note that the same conclusion follows naturally from a classical model of evaporative cooling [7], where the evaporation rate scales as  $\tau_{\text{ev}}^{-1} \sim n\sigma v_{\text{th}} e^{-\eta}$ , with  $\eta = V_0/k_B T$  the evaporation parameter. Since  $\eta \sim 8$  in typical experiments, the separation of scales between the microscopic thermalization time and the evaporation time always holds.

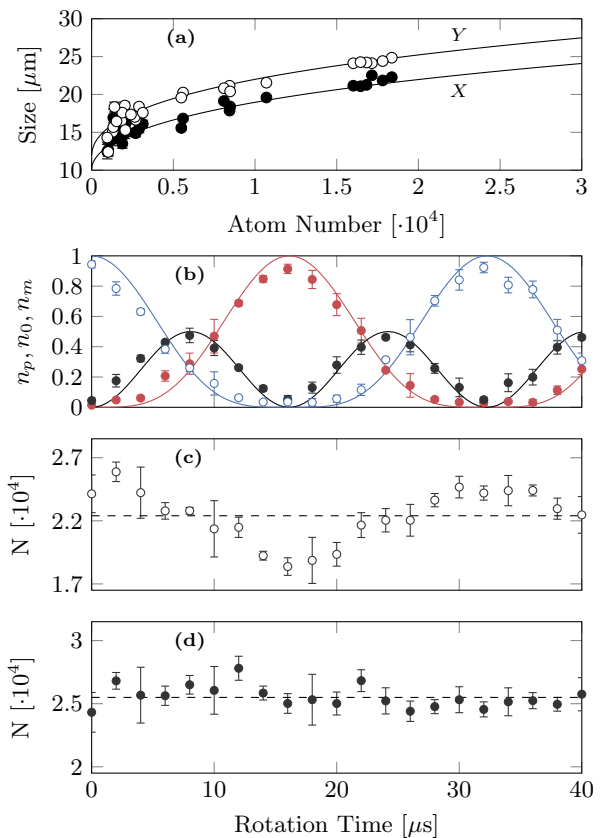

FIG. 5. Calibration of absorption imaging. **a**: Determination of  $\alpha_0$ . Filled and empty symbols stands for the measured Thomas-Fermi sizes along the two trapping axis **X** and **Y**. The solid lines represent the calculated ones. **b**: Normalized Zeeman populations versus rotation time, starting from a cloud initially polarized in  $m_F = +1$ . Filled red symbols stands for  $m_F = +1$ , filled black symbols for  $m_F = 0$  and empty blue symbols for  $m_F = -1$ . **c**: The uncorrected atom number displays an oscillation at the Rabi frequency. **d**: Apart from shot-to-shot variations, the post-calibrated atom number remains constant during the Rabi oscillation.

### III. IMAGE ANALYSIS

#### A. Model and calibration of the scattering cross-sections

For a two-level atom, the atomic column density  $\tilde{n} = \int n(\mathbf{r}) dz$  integrated along the probe line of sight  $z$  can be obtained from

$$\tilde{n} = -\frac{1}{\sigma_0} \left( \log \left( \frac{I_1}{I_2} \right) + \frac{I_1 - I_2}{I_{\text{sat}}} \right), \quad (1)$$

where  $\sigma_0$  is the resonant absorption cross-section,  $I_{\text{sat}}$  the saturation intensity, and  $I_1$  and  $I_2$  refer to the intensity profiles with and without atoms, respectively.

The multilevel structure of real atoms makes the analysis of light scattering in experiments more complicated than Eq. (1) suggests. The number of scattered photons

per atoms will depend not only on the initial internal state, but also on the repumping and probe light polarizations, on the detailed dynamics of the repumping pulse, etc. Computing an effective cross-section for a real experiment would require a detailed modeling of the sequence, presumably very sensitive to errors due to imperfect characterization of the polarizations and spatial modes of the lasers.

Here we use an heuristic extension of the two-level atom model. We assume the column density  $\tilde{n}_{m_F}$  for the Zeeman component  $m_F$  can be written as

$$\tilde{n}_{m_F} = -\frac{\alpha_{m_F}}{\sigma_0} \left( \log \left( \frac{I_1}{I_2} \right) + \frac{I_1 - I_2}{I_{\text{sat}}} \right), \quad (2)$$

with  $\alpha_{m_F}$  a coefficient to be determined. We calibrate the saturation intensity  $I_{\text{sat}}$  as in [8]. In this work, we typically use probe intensities  $\sim 0.1 I_{\text{sat}}$  so that the second term in Eq. (2) is a small correction to the column density. We determine the coefficients  $\alpha_{m_F}$  in two steps. First, we obtain the  $\alpha_0$  coefficient based on measurements of the BEC size vs atom number. To do this, we prepare equilibrium, spin-polarized condensates in  $m_F = 0$  by distilling out  $m_F = \pm 1$  atoms with a magnetic field gradient. We obtain the sizes of the condensate after a time of flight using a Thomas-Fermi fit, and compare our measurements to Gross-Pitaevskii calculations [4]. The calculated sizes, which increase with  $N$  for repulsive interactions, are found by solving numerically the three-dimensional Gross-Pitaevskii equation and performing the aforementioned Thomas-Fermi fit to the simulated data. We obtain the value of  $\alpha_0$  by matching the measured and expected sizes.

In a second step (Fig. 5 b-c), we determine the ratios  $\alpha_{+1}/\alpha_0$  and  $\alpha_{-1}/\alpha_0$  by driving Rabi oscillations between the Zeeman states using a resonant radiofrequency [2]. We adjust the ratios  $\alpha_0/\alpha_{+1}$  and  $\alpha_{-1}/\alpha_{+1}$  and the Rabi Frequency  $\Omega$  to fit the relative population ( $n_{+1,0,-1}$ ). Fig. 5c shows that the total atom number oscillates at the Rabi frequency before correction, and is almost constant (with some residual fluctuations) after correction.

#### IV. EXTRACTING $T_c$

##### A. Bimodal fits

We model the measured column densities using the standard parametrization, *i.e.* by the sum of a Bose-Einstein distribution describing the thermal component and a Thomas-Fermi profile describing the condensate [9]. We fit the three Zeeman components simultaneously, with a few assumptions to reduce the number of fitting parameters. We assume in particular a fugacity  $z = 1$ , equal temperatures for all three thermal clouds, and equal condensate sizes in accordance with the single-mode approximation. From the fit parameters, one can obtain in principle the temperature, the total population

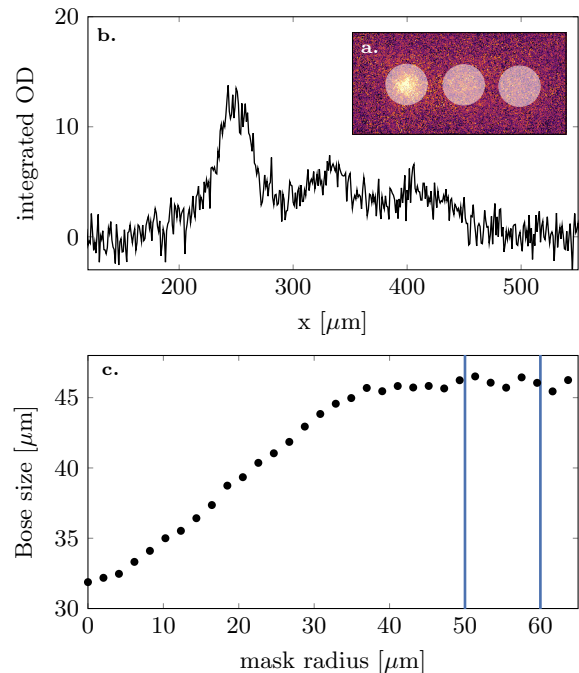

FIG. 6. Extraction of the temperature by fitting thermal density profiles to images with a varying mask sizes. **a**: Typical single shot image with a mask of radius  $30 \mu\text{m}$ . **b**: Integrated density profile from image **a**. **c**: Size of the fitted Bose distributions versus mask size. The final thermal size is obtained by an average over the “plateau” delimited by the vertical blue lines. For mask sizes larger than  $\geq 70 \mu\text{m}$ , the fit fails because imaging noise overtakes the atomic signal. For mask sizes below  $40 \mu\text{m}$ , condensed atoms still contribute to the masked image.

and the condensate fraction of each component. However, the parametrization is heuristic and prone to systematic errors. The bimodal fit is sensitive to image noise when the condensate fraction is below 5%. Additionally, systematic deviations from the Thomas-Fermi profile due to the tight confinement become problematic when the condensate fraction is higher than approximately 50% [1]. For this reason, we only use the bimodal fits to obtain the total populations of each component and the geometric center of each cloud, and use other methods which we believe more reliable to determine the temperature and the critical point.

##### B. Determination of the temperature from the thermal tails of the atomic distribution

We extract the temperature from the wings of the thermal components. The basic assumption is that the wings of the time-of-flight distribution are determined by the wings of the in-trap momentum distribution, which is well approximated by an ideal Bose-Einstein distribution for large enough momenta. To determine the range of momenta where this description applies, we apply circu-

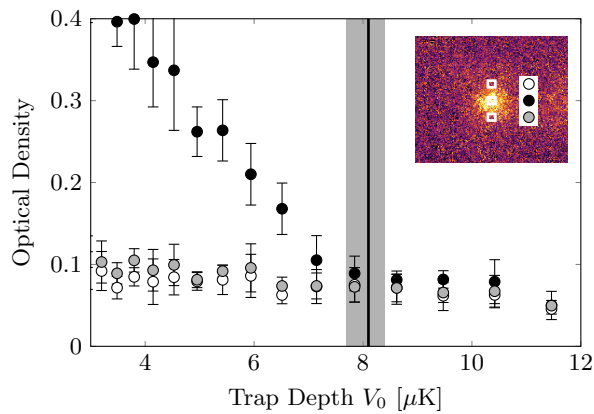

FIG. 7. Optical density as a function of evaporation time, showing the increase of optical density at the BEC transition happens only in the center of the momentum distribution. The inset shows the correspondence between plot symbols and integration regions. The black line shows the Bose-Einstein transition extracted from a fit to the data, and the gray area the 66 % confidence interval.

lar masks at the center of each cloud, as shown in Fig. 6 a, and fit the outer atomic distribution with a Bose-Einstein distribution  $\propto g_2 \left[ e^{-r^2/R_{\text{th}}^2} \right]$ , where  $g_n(x) = \sum_{k=1}^{\infty} x^k/k^n$  is a Bose-Einstein function. The fitted size varies when the size of the mask increases, and eventually reaches a plateau (Fig. 6 c). We identify this plateau with the dilute wings of the cloud, well reproduced by an ideal Bose-Einstein distribution. We extract the temperature from  $k_B T = m R_{\text{plateau}}^2/t^2$ , with  $t$  the time of flight and where  $R_{\text{plateau}}$  is the average of  $R_{\text{th}}$  for five mask sizes between 50  $\mu\text{m}$  and 60  $\mu\text{m}$ .

### C. Determination of the threshold for Bose-Einstein condensation from the peak density

The critical point is detected by a sudden change in the peak value of the optical density  $OD_{m_F} = \sigma_0 \tilde{n}_{m_F}$  of each Zeeman component  $m_F$ . We choose a square integration zone of side  $3 \times 3$  pixels near the center of each component to evaluate the peak optical density. The evolution of  $OD_{+1}$  as a function of evaporation time is shown in Fig. 7, and shows an abrupt change at a particular trap depth which we identify as critical point. We extract the critical trap depth from a piece-wise linear fit to the data near the critical point. Finally, we use the critical trap depth determined to evaluate the atom number, temperature, magnetization and trap frequency (see Fig. 4) at the critical point. Typical statistical uncertainties on the temperature and atom number determined in this way are evaluated to  $\pm 10\%$  and  $\pm 7\%$ , respectively ( $1/e$  confidence intervals). Additionally, we estimate a possible systematic error around 10 % on the calibration of the atom numbers. This has only a small effect on the calculated critical temperature  $T_{c,\text{id}} \propto \bar{\omega} N^{1/3}$  for single-

component ideal gases used as a reference scale in the paper (errors on  $\bar{\omega}$  are negligible).

We have verified that the sudden increase of the optical density is observed only in the center of the distribution. Choosing other off-centered regions is compatible with the behavior of a slowly cooling thermal gas (see Figure 7).

## V. THEORETICAL MODELS OF SPINOR GASES AT FINITE TEMPERATURES

### A. Ideal spin 1 gas

We first calculate the BEC critical temperature of a spin 1 Bose gas with fixed magnetization  $M_z$  and atom number  $N$  [10–12]. The gas is trapped in a harmonic potential with frequencies  $\omega_i$  ( $i = x, y, z$ ). The Gibbs free energy is written as

$$G = H_{\text{sp}} - \sum_{m_F=0,\pm 1} \mu_{m_F} N_{m_F}, \quad (3)$$

with  $H_{\text{sp}}$  the sum of the kinetic and potential energies,  $N_{m_F}$  the population of Zeeman state  $m_F$ , and  $q$  the quadratic Zeeman energy. The chemical potentials for each Zeeman component are given by  $\mu_{\pm 1} = \mu \pm \lambda$  and  $\mu_0 = \mu + q$ , where the Lagrange multipliers  $\mu$  and  $\lambda$  ensure conservation of  $N$  and  $M_z$  on average.

Following the usual method [4], we write the Zeeman population  $N_{m_F} = N_{c,m_F} + N'_{m_F}$  as the sum of the population of the trap ground state  $N_{c,m_F}$  and of all excited state  $N'_{m_F}$ . Here and in the following, the prime subscript denotes quantities related to non condensed atoms. We calculate  $N'_{m_F}$  from the semi-classical formula [13],  $N'_{m_F} = (k_B T / \hbar \bar{\omega})^3 g_3(e^{\beta \mu_{m_F}})$ , with  $\bar{\omega} = (\prod_{i=x,y,z} \omega_i)^{1/3}$ . For a given  $T$ ,  $m_z$  and  $q$ , we find numerically the chemical potential  $\mu$  and  $\lambda$  by solving the set of equations  $\sum_{m_F} N_{m_F} = N$  and  $N_{+1} - N_{-1} = M_z$ .

The BEC transition takes place in the Zeeman component  $m_F$  when  $\mu_{m_F} = 0$ . As the temperature is lowered, the Zeeman components condense sequentially. Ideal gas theory predicts critical temperatures shown as dashed lines in Fig. 8. For  $q > 0$ , there are two regimes depending on the magnetization. For low  $m_z$ , the  $m_F = 0$  component condenses first at a critical temperature  $T_{c1}$ , and the  $m_F = +1$  component condenses second at a lower critical temperature  $T_{c2} \leq T_{c1}$ . For high  $m_z$ , the sequence is reversed. We remark that the  $m_F = -1$  component never condenses, except in the limiting case  $q = 0$  where it condenses simultaneously with  $m_F = 0$ . The conditions on the chemical potentials for each condensation temperature are summarized in Table I.

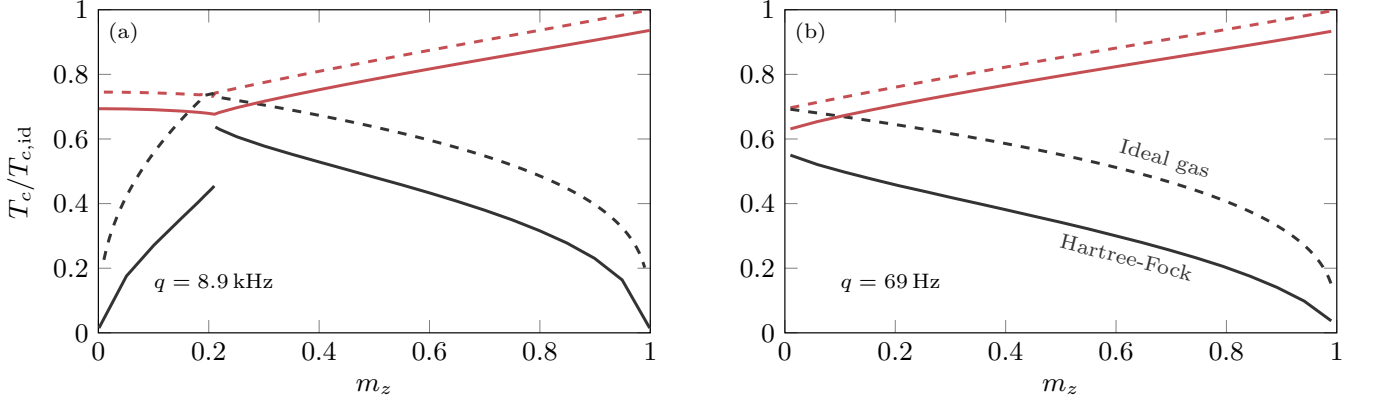

FIG. 8. **a.** Critical temperatures for  $q/h = 8.9 \text{ kHz}$  for  $N = 5 \cdot 10^4$ ,  $\omega = 2\pi \times 1200 \text{ s}^{-1}$ . The red and blue lines show  $T_{c1}$  and  $T_{c2}$ , respectively. The solid lines are calculated using the Hartree-Fock model and the dashed lines using ideal gas theory. The and  $q/h = 69 \text{ Hz}$  **b.** Close-up view of the region near  $m_z^*$  where  $T_{c1}$  and  $T_{c2}$  cross for the ideal gas. The dashed line show the prediction of a so-called “semi-ideal” model intermediate between the ideal gas and the complete Hartree-Fock treatment.

| Condensation order | $m_F = +1$ first                                          | $m_F = 0$ first                                                      |
|--------------------|-----------------------------------------------------------|----------------------------------------------------------------------|
| $T_{c1}$           | $\mu_{+1} = 0$<br>$\mu_0 = q - \lambda$<br>$\mu_{-1} = 0$ | $\mu_{+1} = \lambda - q$<br>$\mu_0 = 0$<br>$\mu_{-1} = -\lambda - q$ |
| $T_{c2}$           | $\mu_{+1} = 0$<br>$\mu_0 = 0$<br>$\mu_{-1} = -2q$         | $\mu_{+1} = 0$<br>$\mu_0 = 0$<br>$\mu_{-1} = -2q$                    |

TABLE I. Summary of the conditions of condensation in the ideal case. Here  $T_{c1/2}$  denotes the first/second critical temperature,  $\mu_{m_F}$  is the effective chemical potential for the Zeeman component  $m_F$ ,  $\lambda$  is a Lagrange multiplier enforcing a given magnetization and  $q$  is the quadratic Zeeman energy. Note that  $\lambda > 0$  when  $m_z > 0$ .

### B. Hartree-Fock model

We now consider the effect of interactions, described by the Hamiltonian [14]

$$\hat{H}_{\text{int}} = \frac{\bar{g}}{2} \int d^3\mathbf{r} \hat{n}^2(\mathbf{r}) + \frac{g_s}{2} \int d^3\mathbf{r} \hat{\mathbf{S}}^2(\mathbf{r}). \quad (4)$$

Here  $\hat{n}_{m_F}(\mathbf{r})$  denotes the spatial density of the  $m_F$  component,  $\hat{n}(\mathbf{r}) = \sum_{m_F} \hat{n}_{m_F}(\mathbf{r})$  the total density, and  $\hat{\mathbf{S}}$  the spin density. In the following we also note  $n'_{m_F}(\mathbf{r})$  the density of non-condensed atoms in state  $m_F$ , and the total non-condensed density  $n'(\mathbf{r}) = \sum_{m_F} n_{m_F}(\mathbf{r})$ .

We make a series of approximations to simplify the problem and compute the thermodynamic properties:

1. We treat the interactions in the Hartree-Fock approximation [15–17],
2. We neglect the spin-dependent interaction term  $\propto g_s$  in comparison with the spin-independent interactions  $\propto \bar{g}$ ,

3. We assume that a semi-classical approximation (for the condensate and for the excited atoms) is valid.

We restrict ourselves to a regime where at most one Zeeman component condenses. This component is identified by the label  $c$  in the following.

Under these assumptions, the density profile of the condensate is determined by

$$n_c(\mathbf{r}) = \frac{1}{\bar{g}} \max \{ \mu_c - V(\mathbf{r}) - \bar{g} [n'(\mathbf{r}) + n'_c(\mathbf{r})], 0 \}, \quad (5)$$

with a BEC index  $c$  corresponding to 0 or +1 depending on the particular case under consideration. The last term describe interactions between condensed and non-condensed atoms, with a strength  $2\bar{g}$  for atoms in the same Zeeman component  $c$  as the condensate and  $\bar{g}$  otherwise. The density profiles of the thermal components are determined by the set of non-linear equations,

$$n'_{m_F}(\mathbf{r}) = \frac{1}{\lambda_T^3} g_{3/2} \left\{ e^{\beta [\mu_{m_F} - W_{m_F}(\mathbf{r})]} \right\}. \quad (6)$$

Here  $W_{m_F}$  denotes a self-consistent mean-field potential for non-condensed atoms in the Zeeman state  $m_F$ ,

$$W_{m_F} = \bar{g} [(1 + \delta_{m_F,c})n_c + n' + n'_{m_F}] + V. \quad (7)$$

Eqs. (5,6) must be solved self-consistently for the thermodynamic potentials parameters  $\mu, \eta$ , imposing the constraints of total atom number and magnetization.

At first sight, it may seem straightforward to extend the model discussed above to include more than one condensed component and spin-dependent interactions terms  $\propto g_s$ . However, antiferromagnetic interactions tend to induce phase separation when  $m_F = 0$  and  $m_F = \pm 1$  are simultaneously condensed [10, 18]. In the experiment, this trend is penalized by the high energetic cost of domain walls in a tight trap, stabilizing a condensate in a single spatial mode. This effect is due to

the so-called “quantum pressure” term neglected in the semi-classical approximation. To include it in a consistent manner, one would need to solve the complete Gross-Pitaevskii equation as well as Schrödinger-like equations for the excited modes in a self-consistent manner. We did not attempt to do such a calculation, which promises to be numerically taxing in three dimensions.

### C. Scaling properties of the Hartree-Fock model

The simplified Hartree-Fock model of Section VB admits a scaling form. We introduce the critical temperature of a single component ideal gas,  $k_B T_{c,id} = \hbar\bar{\omega}(N/\zeta(3))^{1/3}$ , and two associated spatial scales, the thermal De Broglie wavelength  $\lambda_{c,id} = (2\pi\hbar^2/mk_B T_{c,id})^{1/2}$  and the thermal cloud radius  $R_{c,id} = (k_B T_{c,id}/m\omega^2)^{1/2}$ . We now introduce dimensionless variables denoted with a tilde symbol. Energies are scaled by  $T_{c,id}$ , and densities by  $1/\lambda_{c,id}^3$ . With these notations, any thermodynamic state function can be rewritten as universal functions of the scaled temperature  $\tilde{T}$ , chemical potentials  $\tilde{\mu}, \tilde{\eta}$  and quadratic Zeeman energy  $\tilde{q}$ , and of the dimensionless strength of interactions  $\gamma$

$$\gamma = \frac{\bar{g}}{\lambda_{c,id}^3 k_B T_{c,id}} = \frac{2\bar{a}}{\lambda_{c,id}}. \quad (8)$$

This is a natural extension of the scaling behavior noted for single-component Bose gases [13]. In three dimensions, this behavior holds because of the semi-classical approximation. Including the kinetic energy in the theory would break the universality.

### D. Example of results from the Hartree-Fock model

As an example, the calculated critical temperature for  $g/h = 8.9$  kHz is shown in Fig. 8a for fixed atom number and trap frequencies. One observes a significant shift downwards of the interacting model from the non-interacting one, as expected for repulsive interactions [15].

In the ideal gas model, the critical temperature curves  $T_{c,1}$  and  $T_{c,2}$  are continuous and cross at a particular point labeled as  $m_z^*$ . In contrast, the Hartree-Fock model shows a discontinuity of the second critical temperature near  $m_z^*$ . To understand this feature, we turn to a “semi-ideal model”, which is simpler to discuss but preserves the discontinuity (Fig. 8b). In the semi-ideal model [19], one retains only terms proportional to  $\bar{g}n_c$  and neglects terms proportional to  $\bar{g}n'_{m_F}$  in Eqs. (5,6). Uncondensed atoms experience a mean-field potential which differs from the harmonic trapping potential only within the volume of the condensate, and depends on their internal state : either a  $W$ -shaped potential for atoms in the same Zeeman state the condensate (similar to the

single-component case [19]) or a “flat-bottom” potential for atoms in other Zeeman states [20, 21].

To explain the discontinuity of  $T_{c,2}$ , we consider the temperature regime  $T_{c,1} > T > T_{c,2}$ , and the case  $m_z < m_z^*$  first. The condensate forms in  $m_F = 0$ , and the magnetization is entirely carried by the thermal component ( $N'_{+1} - N'_{-1} = M_z$ ). The condition for second condensation is  $\mu_{+1} = \mu + \lambda = \bar{g}n_c(\mathbf{0})$ , with  $n_c(\mathbf{0})$  the condensate density in the center of the trap. Since  $\mu_0 = \mu + q = \bar{g}n_c(\mathbf{0})$ , this leads to the same condensation criterion  $\lambda = q$  as for an ideal gas. Lowering the temperature leads to both a decrease of the total thermal population  $N' = N'_0 + N'_{+1} + N'_{-1}$  and an increase in the degree of polarization of the thermal component,  $P'_z = (N'_{+1} - N'_{-1})/N'$ . Note that mean-field interactions compared to the one of an ideal gas at the same temperature  $T$  and chemical potential  $\lambda < q$ . For “high” temperatures  $T \lesssim T_{c,1}$ , when the condensate population is small ( $N' \sim N$ ), the conservation of magnetization amounts to  $m_z \approx P'_z$ . The flattening of the mean-field potential for uncondensed  $m_F = \pm 1$  atoms leads to a slight increase of the atom number  $N_{c,m_F}$  at which these Zeeman components can condense. Equivalently, the chemical potential  $\lambda$  must adjust to a value  $< q$  in order to maintain a given magnetization. This effect prevents condensation in  $m_F = +1$  in a wide temperature range, until the condensate population becomes sufficiently large. In that regime, the conservation law  $m_z = P'_z \times N'/N$  is fulfilled if the decrease of  $N'/N$  is compensated by an increase of  $P'_z$ . This corresponds to an increase of  $\lambda$  which eventually reaches the critical value  $\lambda = q$ . As a consequence, the formation of a condensate in the minority component  $m_F = +1$  is delayed to low temperatures, when the condensed fraction in  $m_F = 0$  is large enough.

In the other case  $m_z \gtrsim m_z^*$ , the BEC first appears in the  $m_F = +1$  component. The magnetization is now shared between the condensate and the thermal component, and  $m_z = N_c/N + P'_z \times N'/N$ . As the temperature decreases and the condensate population in  $m_F = +1$  increases, the conservation of  $m_z$  is ensured by decreasing  $N'_{+1}$  and increasing  $N'_0$ . As a result, the condensation in  $m_F = 0$  is not merely shifted to lower values by the mean-field potential. The shift depends on the condensate population at  $T_{c,2}$  and vanishes for  $m_z = m_z^*$  in the semi-ideal model.

The explanation of the discontinuity in the more complete Hartree-Fock theory is qualitatively the same in the semi-ideal model.

### E. Comparison with experimental data

In order to make a comparison of the Hartree-Fock model with the experimental data, we need to account for the variations of the parameters  $N, \omega$  across all data. These parameters naturally decrease while the evaporation ramp proceeds to lower temperatures. As a result, for a given evaporation trajectory  $N, \omega$  are smaller at

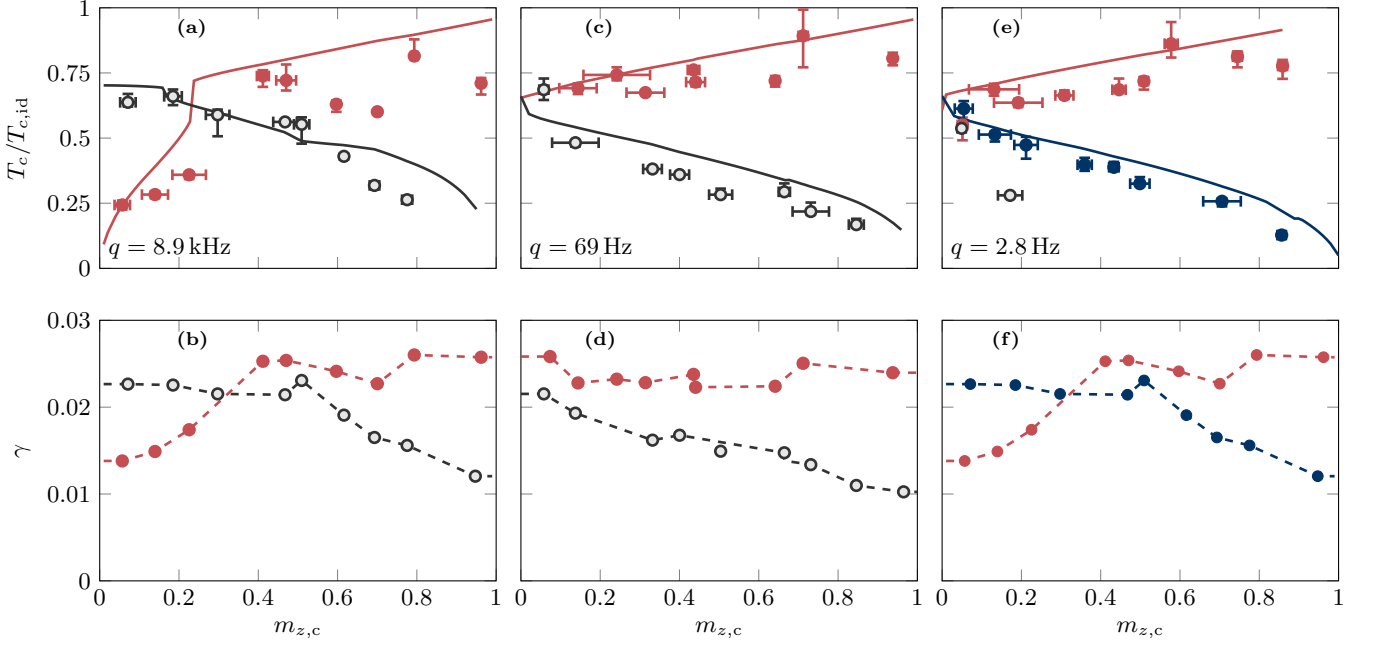

FIG. 9. Comparison between the experimental data and the Hartree Fock model for  $q/h = 8.9$  kHz (a,b),  $q/h = 69$  Hz (c,d), and  $q/h = 2.8$  Hz (e,f). For each column, the top panel shows the critical temperatures. The bottom panel shows the value of the interaction parameter  $\gamma$  for each measured critical temperature (circles), as well as the interpolated curves  $\gamma(m_z)$  used as input for the Hartree-Fock calculation (dashed lines). In each panel, red, gray and dark blue colors correspond to  $m_F = +1$ ,  $m_F = 0$  and  $m_F = -1$ , respectively.

the second critical temperature than at the first. Additionally, the magnetization varies as well as evaporation proceeds (see Sec. II B). Instead of a couple of critical temperatures  $T_{c1}, T_{c2}$  for given  $m_z, N, \omega$ , we have in fact two sets of parameters  $(T_{c1}, m_{z1}, N_1, \omega_1)$  and  $(T_{c2}, m_{z2}, N_2, \omega_2)$ .

One possibility is to do a point-by-point comparison. This results in a sparsely sampled curve that does not reflect the full behavior of the critical temperatures. To cure this, we have performed an interpolation of the experimental parameters to use as input in the calculation. We used the scaling properties of the thermodynamic functions discussed in Sec. V C. We perform a numerical interpolation of the experimentally determined values of  $\gamma$  calculated from Eq. (8), the measured  $T_{c1}$  and  $\bar{g} = 4\pi\hbar^2\bar{a}/m_{\text{Na}}$ . The s-wave scattering length  $\bar{a}$  is measured in [22] and  $m_{\text{Na}}$  is the mass of a sodium atom. We plot the final results in reduced units. The critical temperature curves shown in the main article are reproduced in Fig. 9, together with the measured values of  $\gamma$  and their interpolations.

#### F. Further corrections to the ideal gas critical temperature

*a. Finite-size effects :* The ideal gas theory is computed with the semi-classical formula, valid in the thermodynamic limit for trapped gases [13], *e.g.* when  $N \rightarrow$

$\infty$  and  $\omega \rightarrow 0$  keeping  $N\omega^3$  constant. For finite  $N$  and  $\omega$ , corrections to the thermodynamic limit decrease the critical temperature by  $\delta T_c/T_{c,\text{id}} \simeq -0.73N^{-1/3}$ . This correction is between  $-1\%$  ( $N_c = 10^5$ ) and  $-4\%$  ( $N_c = 10^4$ ) for our experimental parameters.

*b. Trap anharmonicity :* The CDT is only harmonic near its minimum and has a finite trap depth. The most energetic atoms are sensitive to the non-harmonic shape of the CDT potential and also to the finite trap depth (see Fig. 3). The evaporation parameter  $\eta = V_0/k_B T$  remains large ( $\eta > 7$ ) during the evaporation ramp, so that the fraction of atoms affected by these effects is small.

The critical atom number and temperature are affected by two separate effects. First, the finite trap depth introduces an energy cutoff that reduces the critical atom number and increases  $T_c$  (this effect is likely to be enhanced when gravity is taken into account). Second, the anharmonic part of the CDT potential tend to increase  $N_c$  and thus to reduce of  $T_c$  (Gaussian traps are “looser” than pure harmonic traps near their edges). The second effect becomes more important for high values of  $\eta$ .

We have estimated the two effects by evaluating numerically the critical atom number in a CDT potential, using

$$N_c = \int_0^{V_0} \rho(\epsilon) f_{\text{BE}}(\epsilon) d\epsilon, \quad (9)$$

with  $f_{\text{BE}}(\epsilon) = (e^{\beta\epsilon} - 1)^{-1}$  the critical Bose-Einstein distribution and  $\rho(\epsilon)$  the density of states. We have taken

a potential of the form given in Section II A, with beam sizes  $21\,\mu\text{m}$  and  $25\,\mu\text{m}$  for the two arms of the CDT. For an evaporation parameter  $7 < \eta < 10$  as in our experiments, the effect of the anharmonicity is dominant, and we evaluate a reduction of the critical temperature around -3% for  $\eta = 8$ . We did not consider in this calculation atoms possibly trapped in the arm region, which would slightly further the magnitude of the shift.

*c. Combined effect of the finite-size and anharmonicity corrections:* To summarize this Section, the combination of finite-size effects and of the deviation of the CDT potential from an harmonic one can lower the critical temperature of a non-interacting gas by  $\sim -5\%$

compared to the semi-classical prediction in a harmonic trap. The finite-size effects are not easily incorporated in the Hartree-Fock model. Trap anharmonicity effects are difficult to evaluate rigorously due to the ambiguity in the precise definition of the trap depth and of the role of a small, high energy population in the arms of the dipole trap. As a result, we did not include these effects in the comparison between theory and experiments. However, the order-of-magnitude estimate presented here show that they could well explain most of the residual shift between the experimental data and the Hartree-Fock model.

- 
- [1] D. Jacob, L. Shao, V. Corre, T. Zibold, L. De Sarlo, E. Mimoun, J. Dalibard, and F. Gerbier, “Phase diagram of spin-1 antiferromagnetic Bose-Einstein condensates,” *Phys. Rev. A* **86**, 061601 (2012).
  - [2] T. Zibold, V. Corre, C. Frapolli, A. Invernizzi, J. Dalibard, and F. Gerbier, “Spin-nematic order in antiferromagnetic spinor condensates,” *Phys. Rev. A* **93**, 023614 (2016).
  - [3] K. M. O’Hara, M. E. Gehm, S. R. Granade, and J. E. Thomas, “Scaling laws for evaporative cooling in time-dependent optical traps,” *Phys. Rev. A* **64**, 051403 (2001).
  - [4] L. P. Pitaevskii and S. Stringari, *Bose-Einstein condensation* (Oxford University Press, 2003).
  - [5] R. Grimm, M. Weidemüller, and Y. B. Ovchinnikov, “Optical dipole traps for neutral atoms,” (Academic Press, 2000) pp. 95 – 170.
  - [6] H. Wu, E. Arimondo, and C. J. Foot, “Dynamics of evaporative cooling for Bose-Einstein condensation,” *Phys. Rev. A* **56**, 560–569 (1997).
  - [7] O. J. Luiten, M. W. Reynolds, and J. T. M. Walraven, “Kinetic theory of the evaporative cooling of a trapped gas,” *Phys. Rev. A* **53**, 381–389 (1996).
  - [8] G. Reinaudi, T. Lahaye, Z. Wang, and D. Guéry-Odelin, “Strong saturation absorption imaging of dense clouds of ultracold atoms,” *Opt. Lett.* **32**, 3143–3145 (2007).
  - [9] W. Ketterle, D. S. Durfee, and D. M. Stamper-Kurn, “Making, probing and understanding Bose-Einstein condensates,” in *Proceedings of the International School on Physics Enrico Fermi 1998, Bose-Einstein Condensation in Atomic Gases*, edited by M. Inguscio, S. Stringari, and C. E. Wieman (IOS Press, 1999) pp. 67–176, arXiv:cond-mat/9904034.
  - [10] T. Isoshima, T. Ohmi, and K. Machida, “Double phase transitions in magnetized spinor Bose-Einstein condensation,” *Journal of the Physical Society of Japan* **69**, 3864–3869 (2000).
  - [11] W. Zhang, S. Yi, and L. You, “Bose-Einstein condensation of trapped interacting spin-1 atoms,” *Phys. Rev. A* **70**, 043611 (2004).
  - [12] G. Lang and E. Witkowska, “Thermodynamics of a spin-1 Bose gas with fixed magnetization,” *Phys. Rev. A* **90**, 043609 (2014).
  - [13] F. Dalfovo, S. Giorgini, L. P. Pitaevskii, and S. Stringari, “Theory of Bose-Einstein condensation in trapped gases,” *Rev. Mod. Phys.* **71**, 463–512 (1999).
  - [14] D. M. Stamper-Kurn and M. Ueda, “Spinor Bose gases: Symmetries, magnetism, and quantum dynamics,” *Rev. Mod. Phys.* **85**, 1191–1244 (2013).
  - [15] S. Giorgini, L. P. Pitaevskii, and S. Stringari, “Condensate fraction and critical temperature of a trapped interacting Bose gas,” *Phys. Rev. A* **54**, R4633–R4636 (1996).
  - [16] W. Krauth, “Quantum Monte Carlo calculations for a large number of bosons in a harmonic trap,” *Phys. Rev. Lett.* **77**, 3695 (1996).
  - [17] Y. Kawaguchi, N. T. Phuc, and P. B. Blakie, “Finite-temperature phase diagram of a spin-1 Bose gas,” *Phys. Rev. A* **85**, 053611 (2012).
  - [18] S. Yi, Ö. E. Müstecaplıoğlu, C. P. Sun, and L. You, “Single-mode approximation in a spinor-1 atomic condensate,” *Phys. Rev. A* **66**, 011601 (2002).
  - [19] M. Naraschewski and D. M. Stamper-Kurn, “Semi-analytical description of a trapped Bose gas at finite temperature,” *Phys. Rev. A* **58**, 2423 (1998).
  - [20] F. Fang, R. Olf, S. Wu, H. Kadau, and D. M. Stamper-Kurn, “Condensing magnons in a degenerate ferromagnetic spinor Bose gas,” *Phys. Rev. Lett.* **116**, 095301 (2016).
  - [21] C. Klempt, O. Topic, G. Gebreyesus, M. Scherer, T. Henninger, P. Hyllus, W. Ertmer, L. Santos, and J. J. Arlt, “Multiresonant spinor dynamics in a Bose-Einstein condensate,” *Phys. Rev. Lett.* **103**, 195302 (2009).
  - [22] S. Knoop, T. Schuster, R. Scelle, A. Trautmann, J. Appmeier, M. K. Oberthaler, E. Tiesinga, and E. Tiemann, “Feshbach spectroscopy and analysis of the interaction potentials of ultracold sodium,” *Phys. Rev. A* **83**, 042704 (2011).
